# Supplementary material for: An Introduction to Probabilistic Programming
Source: arXiv:1809.10756 source file (2021-10-19)
Supplement: Supplementary file 1 [file appendix-functional-programming.tex]

% !TEX root =  ../single-chapter.tex
% !TEX spellcheck = en_US

The FOPPL and HOPPL are both pure, nearly functional languages (technically \mang{sample} and \mang{observe} are exceptions; \mang{sample} violates referential transparency and \mang{observe} is not side-effect free). Syntactically, both are similar to LISP and borrow directly from Clojure.  

Among other things this means that parenthesis are used for function application.  The first element in a parenthesized sequence is a function (or special form), and the following elements are its arguments.  It can take a few minutes to become accustomed to this sort of so-called ``prefix'' notation.  The following two examples demonstrate evaluation of a series of standard arithmetic and mathematical expressions.

First
\begin{hoppl}[mathescape]
(+ 1 1)
$\Longrightarrow$ 2
\end{hoppl}
applies the function~\mang{+}~to the argument list \mang{1 1} and evaluates to \mang{2}.  And second
\begin{hoppl}[mathescape]
(- 10 3)
$\Longrightarrow$ 7
\end{hoppl}
applies the function~\mang{-}~to the argument list \mang{10 3} which evaluates to \mang{7}. 

This is the main difference to ``infix'' languages.  The expression \mang{(- 10 7)} would, in most infix languages, be written $(10 - 7)$.  Allowing only prefix expressions greatly simplifies translation rules and book presentation of material at the cost of being less readable and intuitive for the majority of human programmers.

For instance, the expression
\begin{hoppl}[mathescape]
(/ (* 10 (+ 2.1 4.3)) 2)
\end{hoppl}
is equivalent to the mathematical expression $(10 \times (2.1 + 4.3) / 2).$

Standard mathematical functions like $\log, \exp,$ and more can be composed and called in the same way, i.e. \mang{(exp -2)}, \mang{(log (+ 1 1))}, and \mang{(sqrt 5)} provided that they are implemented in a standard library using \mang{defn} or are imported from an implementing language.  Throughout the book we assume the existence of a standard library of ``primitive functions'' including standard mathematical functions such as these.

Note that there are no ``types'' syntactically speaking.  We stipulate that HOPPL and FOPPL, like LISP, are dynamically typed and all necessary type conversions, if necessary and possible, are performed by the evaluator at runtime (i.e. floating point number to integer casts, etc.).

Comparison operators (\mang{<}, \mang{>}, \mang{=}, \mang{<=}, \mang{>=}) are functions that return booleans and behave as one would expect.  In particular they can be used in \mang{if} statement predicate expressions . The \mang{if} statement takes the form

\begin{hoppl}[mathescape]
(if predicate-expr 
  expr-if-true 
  expr-if-false)
\end{hoppl}
For instance \mang{(< 4 10) $\Longrightarrow$ true}.   Continuing, this means that
\begin{hoppl}[mathescape]
(if (> 3 2) 1 -1)
$\Longrightarrow$ 1.
\end{hoppl}
Here are a couple more examples of conditional branching:
 \begin{hoppl}[mathescape]
(if (<= 3 3) (+ 10 10) 0)
$\Longrightarrow$ 20
\end{hoppl}
and
\begin{hoppl}[mathescape]
(+ (if (< 4 5) 1 2) 3)
$\Longrightarrow$ 4.
\end{hoppl}
 A \mang{let} block is a critical special form which can be used to define variables within a local scope. A \mang{let} block takes a vector-valued initial argument which defines a sequence of ``bindings,'' followed by a sequence of statements.  Bindings are syntactically a list in square-brackets \mang{[]} of name-value pairs. In \mang{(let [x 1 y 2] expr)}, \mang{expr} is evaluated with \mang{x} set equal to 1, and \mang{y} equal to 2.  If a \mang{let} block includes multiple expressions, the return value of the entire block is the value of the last expression.
 
Some examples of \mang{let} blocks follow:
\begin{hoppl}[mathescape]
(let [x 10
      y 2]
  (+ x y))
$\Longrightarrow$ 12
\end{hoppl}
\begin{hoppl}[mathescape]
(let [x 10
      y 2]
  (* x 3)
  (+ x y))
$\Longrightarrow$ 12
\end{hoppl}
Note here that the expression \mang{(* x 3)} produces no effect on the return value and, in this example, need not even be evaluated.  In the FOPPL and HOPPL, \mang{observe} expressions are often placed in this syntactic position so as to produce an effect on the inference but not the return value so to speak.
\begin{hoppl}[mathescape]
(let [x 10
      y 2]
  (+ (* x 3) y))
$\Longrightarrow$ 32
\end{hoppl}
\begin{hoppl}[mathescape]
(let [x 10
      y 2
      x (* x 3)]
  (+ x y))
$\Longrightarrow$ 32.
\end{hoppl}
Functions can be defined in the FOPPL and are first class objects in the HOPPL.  That stated, the FOPPL explicitly allows defining functions
\begin{hoppl}[mathescape]
(defn my-fn [x y]
  (+ (* 2 x) y))
\end{hoppl}
which can subsequently be used elsewhere, i.e.~\mang{(my-fn 5 9) $\Longrightarrow$ 19}.

The HOPPL is more akin to a typical LISP in that first class functions are supported.  When functions are first class, this means that variables can be function valued.  This is an extremely powerful language facility.  Consider the following, which uses the \mang{fn} keyword to 
define a local function of two arguments, \mang{x} and \mang{y}, within a \mang{let} block scope, and then calls that function
\begin{hoppl}[mathescape]
(let [my-fn (fn [x y] 
              (+ (* 2 x) y))]
  (my-fn 5 9)) 
$\Longrightarrow$ 19.
\end{hoppl}
Chapter~\ref{ch:hoppl} shows how to use first class functions to implement higher-order operations like \mang{map} and \mang{reduce} which accept functions as arguments.  

We follow Clojure in how it deviates slightly from LISP in that it has other primitive datastructures in addition to lists.  We assume implementing language support for \em pure \em list, vector, and hash-map datastructures, along with accessor primitive functions including \mang{first},  \mang{rest}, \mang{last}, \mang{append}, \mang{get}, and so forth (see Chapter~\ref{ch:foppl}).  Being pure means that all getters and setters (e.g.~\mang{put}) return a {\em new} copy of the datastructure; there is no in-place state-modification.  This might seem to be inefficient but modern, pure datastructures are in fact very fast.   Having first class datastructures such as these means that variables in the FOPPL and HOPPL can be list-, vector-, or hash-map- valued and that there are constructor methods for each data-type.  Some examples follow:
\begin{hoppl}[mathescape]
(let [x (list 1 2 3)]
   (append x 4))
$\Longrightarrow$ (1 2 3 4) 
\end{hoppl}
\begin{hoppl}[mathescape]
(let [x (vector 1 2 3 4)
      y (last x)
      z (list (first x))
      a (append z y)]
  (+ (first a) (first (rest a))))
$\Longrightarrow$ 5
\end{hoppl}

The expressive power of a language like the HOPPL can be surprising to those not already accustomed to functional programming.  Without question the bible for those wishing to grow a deeper understanding of what can be accomplished using such languages is \citetitle{sicp} by \citet{sicp}.  We highly recommended the interested reader to it.
